# Supplementary material for: FloatingFusion: Depth from ToF and Image-stabilized Stereo Cameras
Source: arXiv:2210.02785 source file (2022-10-06)
Supplement: Supplementary file 1 [file appendix.tex]

\appendix
\section{Appendix}
\label{sec:appendix}

\subsection{Metrics}
For depth evaluation, we use the following metrics:
\begin{itemize}
    \item MAE: $\frac{1}{n}\sum |d - d^*|$
    \item RMSE: $\sqrt{\frac{1}{n}\sum (d - d^*)^2}$
    \item MAE Rel.: $\frac{1}{n}\sum |d - d^*|/d^*$
    \item RMSE Rel.: $\sqrt{\frac{1}{n}\sum \left((d - d^*)/d^*\right)^2}$
    \item Bad ratio: percentage of pixel with error $|d - d^*|$ above threshold
\end{itemize}
with $d$ the estimated depth, $d^*$ ground truth, $n$ the number of valid pixels.

\subsection{Implementation Details}
\mparagraph{Fusion training}
We initialize $\tau=140$ and the RAFT-stereo weights using Middlebury checkpoints. For training, we run 10k iteration with a batch size of 4 and a crop size of 640$\times$1440 pixels.

\mparagraph{Mip-NeRF optimization}
The ToF depth loss is scaled by an exponential decay $N_0\exp^{-\lambda i / m}$ where $N_0=10$, $\lambda=8$, $i$ is the current iteration and $m$ is the total number of iterations.
We train Mip-NeRF for 200k iterations and a batch size of 4096 rays.

\subsection{Additional Results}

\NEW{
\mparagraph{Additional Scenes}
Figure~\ref{fig:snapshot_comparison_2} shows more ToF/stereo fusion results captured with our phone.

\mparagraph{Input ToF}
Figure~\ref{fig:tof_vs_ours} shows the depth estimated from the ToF sensor and our fusion results. Depth from ToF is much noisier and lower resolution, with blurry depth edges.
}

\begin{figure}[htp]
	\centering
	\resizebox{\columnwidth}{!}{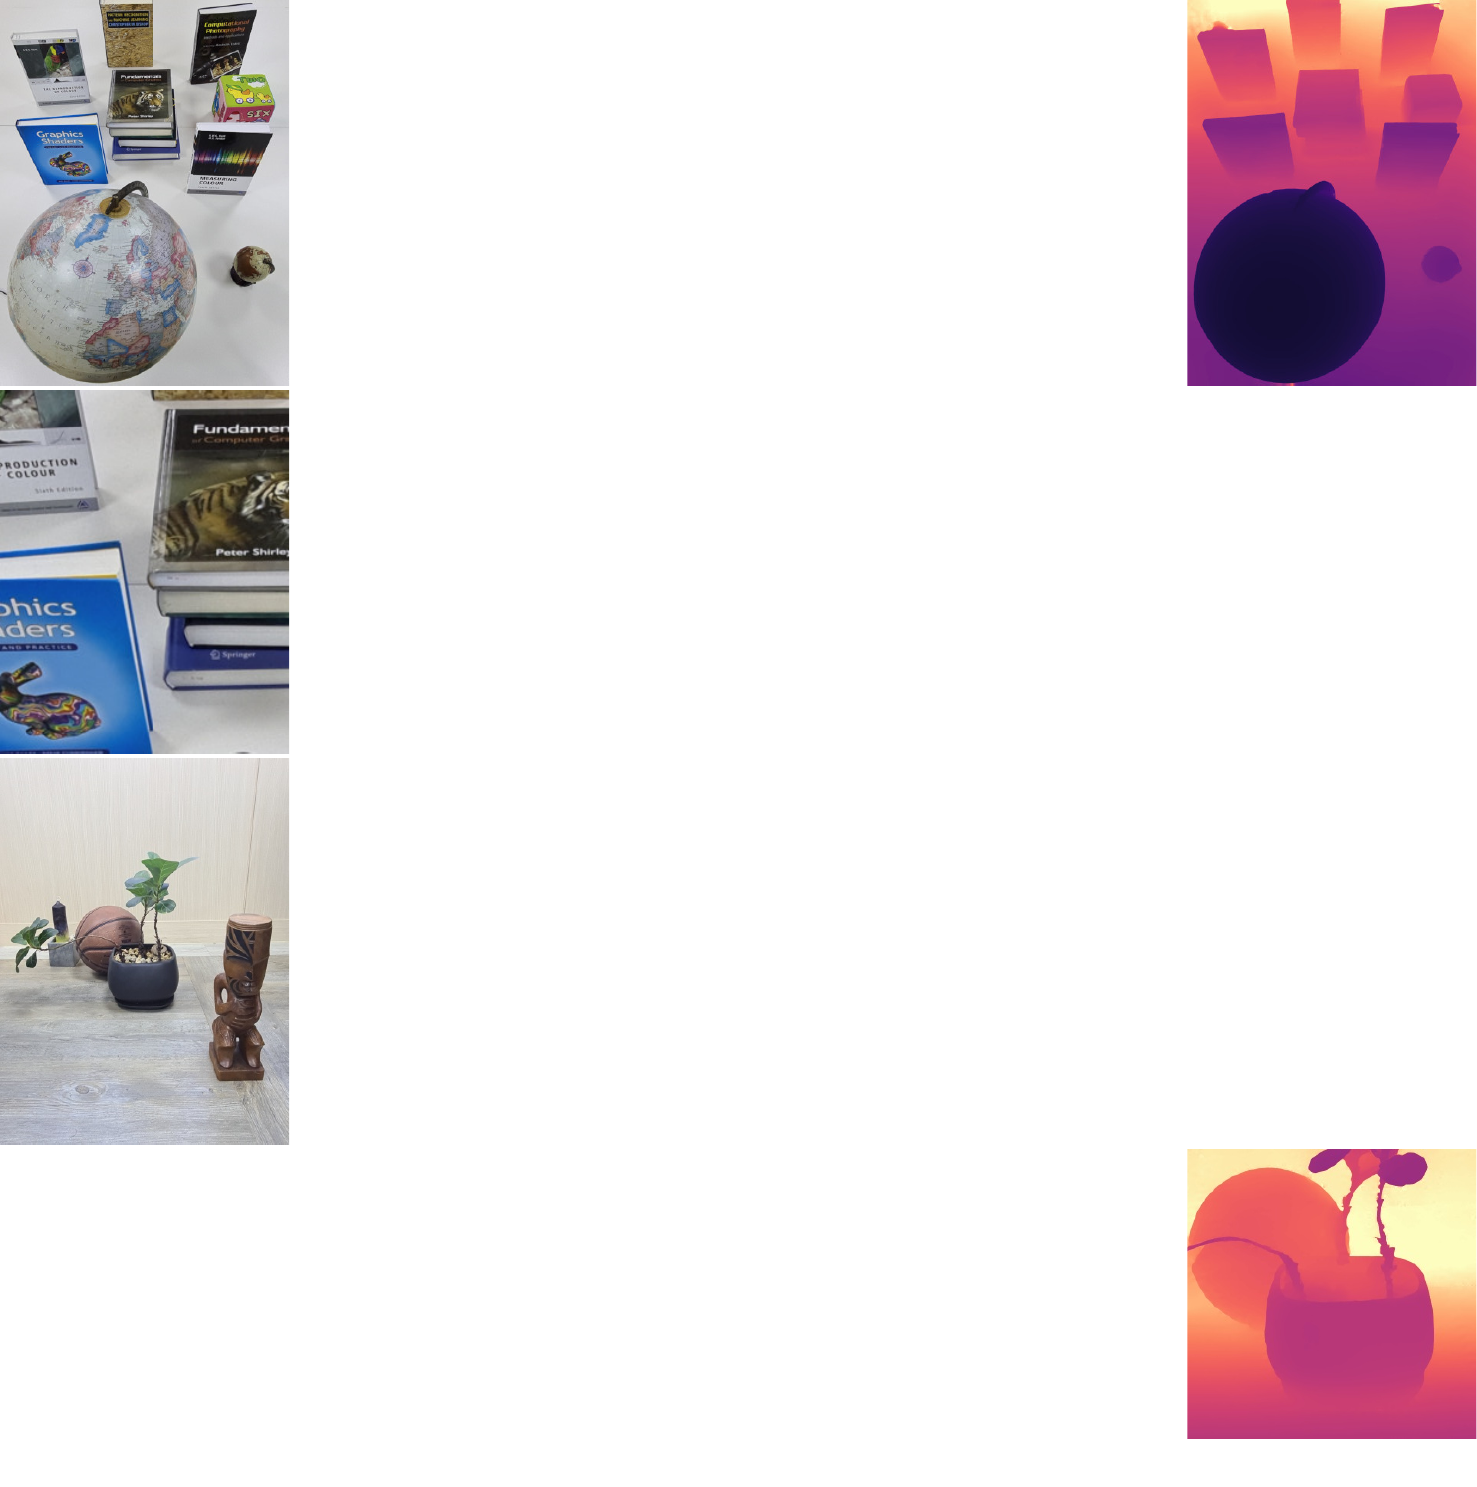}
\caption{\label{fig:snapshot_comparison_2}
		\NEW{Additional mobile ToF/stereo fusion results.}
	}
\end{figure}

\begin{figure}[htp]
	\centering
	\resizebox{\columnwidth}{!}{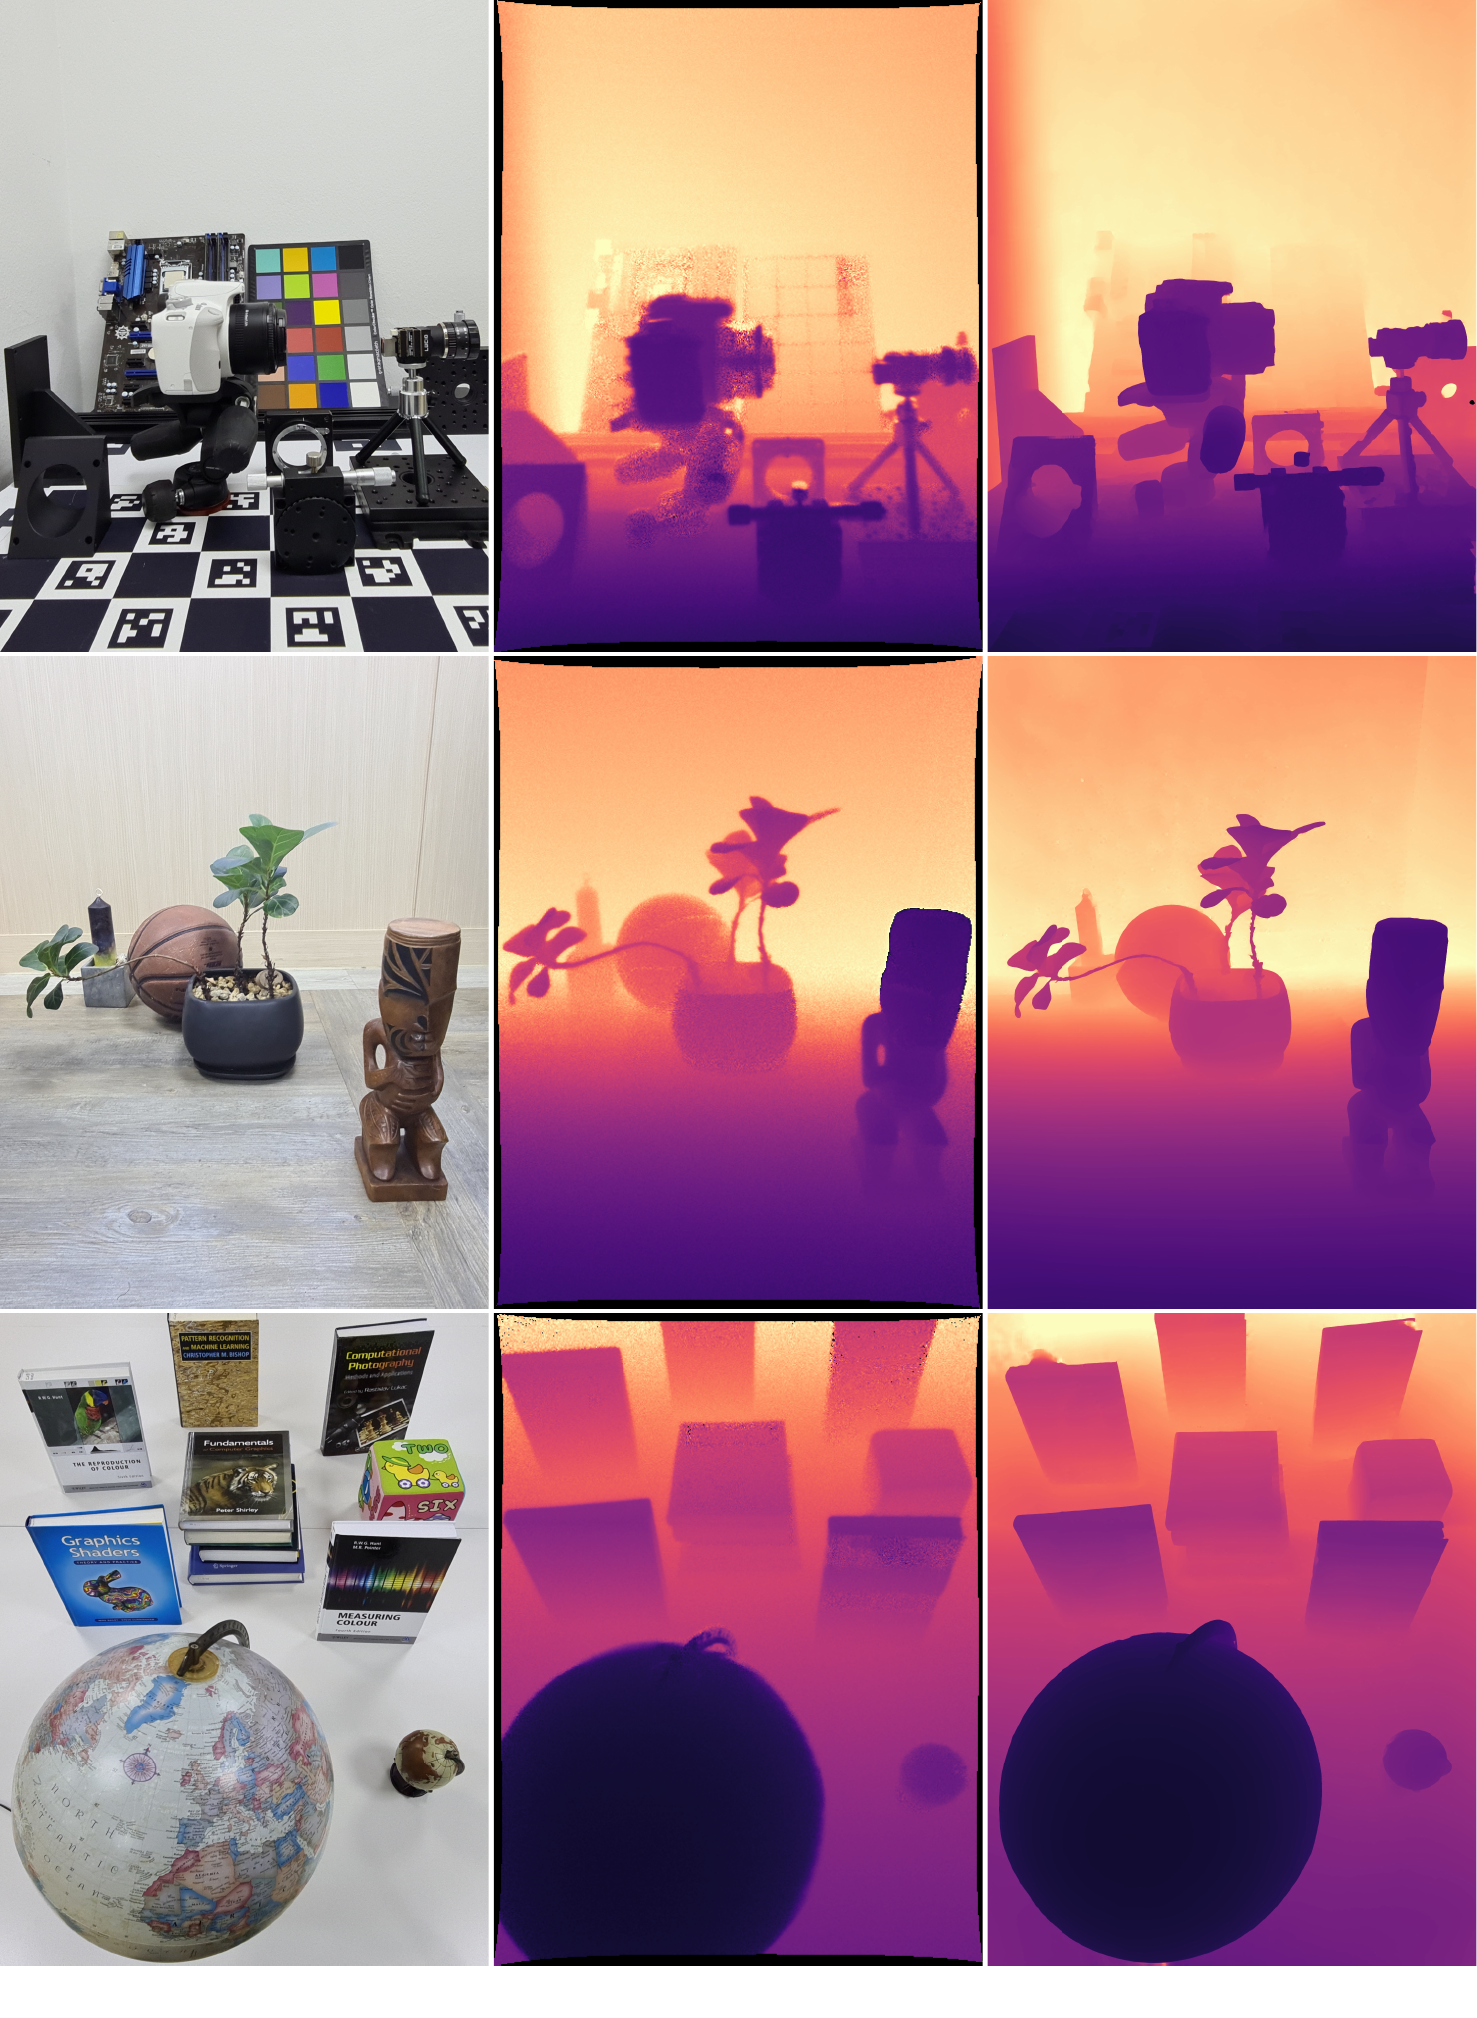}
	\caption{\label{fig:tof_vs_ours}
		\NEW{Input ToF depth and our fusion results.}
	}
\end{figure}

\begin{figure}[htbp]
	\centering
	\resizebox{0.75\columnwidth}{!}{\input{figs/synth3.pdf_tex}}
	\caption{\label{fig:synth3}
        Our ToF/stereo fusion results on the rendered SYNTH3 dataset \cite{agresti2017fusion}. 
	}
\end{figure}

\begin{figure}[htbp]
	\centering
	\resizebox{\columnwidth}{!}{\input{figs/real3.pdf_tex}}
	\caption{\label{fig:real3}
        Our ToF/stereo fusion results on REAL3 dataset \cite{agresti2019fusion_synthetic}. 
	}
\end{figure}

\begin{figure}[htbp]
	\centering
	\resizebox{\columnwidth}{!}{\input{figs/lttm5.pdf_tex}}
	\caption{\label{fig:lttm5}
        Our ToF/stereo fusion results on LTTM5 dataset \cite{mutto2015probabilisticFusion}. 
	}
\end{figure}

\begin{figure}[htbp]
	\centering
	\resizebox{\columnwidth}{!}{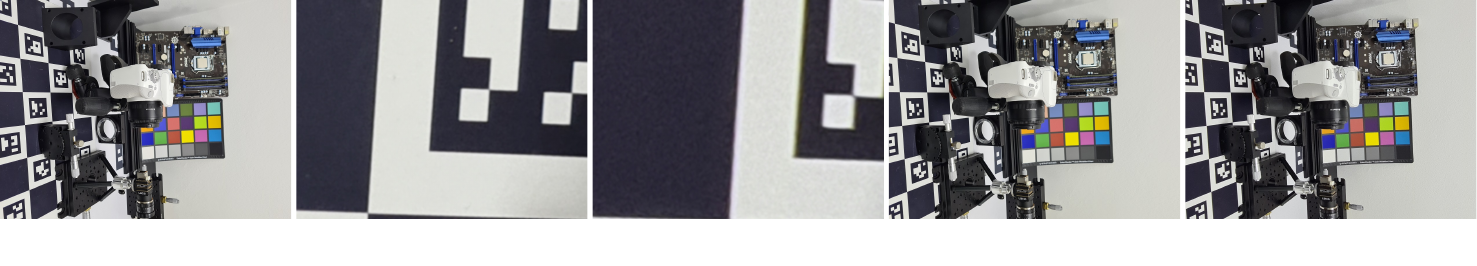}
    \vspace{-5mm}
	\caption{\label{fig:calibration_failure}
        \NEW{Estimating innacurate calibration parameters can lead to poor rectification. (b) rectifying the stereo pair based on Gao et al.~\cite{gao2017selfcalibratingtof}'s approach aggressively crops the images and they are not horizontally aligned (see the vertical shift of the checkerboard corner). (c) Our calibration provides more sensible results and the images of stereo pair are aligned.}
	}
\end{figure}

\begin{table}[t]
	\centering
	\caption{\label{tab:fusion_comparison}
    Disparity error of stereo+ToF fusion techniques. Reported numbers are from respective works, except for $\dagger$ that have been evaluated in \cite{agresti2019fusion_synthetic}. Our method outperforms others on the real-world datasets REAL3 \cite{agresti2019fusion_synthetic} and LTTM5 \cite{mutto2015probabilisticFusion}. \NEW{We show the results of guided ToF upsampling as ``Interpolated ToF'' for reference.} 
	}
    \begin{tabular}{l rr rr rr}
        \toprule
        & \multicolumn{2}{c}{SYNTH3} & \multicolumn{2}{c}{REAL3} & \multicolumn{2}{c}{LTTM5} \\
        & MAE & MSE & MAE & MSE & MAE & MSE \\
        \midrule
        \NEW{Interpolated ToF~\cite{agresti2019fusion_synthetic}} & 0.66 & 4.75 & 2.55 & 10.76 & 1.53 & 11.68 \\
        Marin et al.~\cite{Marin2016ReliableFO}$^\dagger$ & 0.64 & 4.20 & 2.19 & 8.82 & 1.15 & 7.67 \\
        Agresti et al.~\cite{agresti2019fusion_synthetic} & 0.53 & 3.92 & 1.65 & 8.35 & 0.89 & 7.40 \\
        Deng et al. \cite{yong2021fusion} & 0.30 & \textBF{1.84} & 0.93 & 5.84 & 0.79 & 3.47 \\
        Dal Mutto et al. \cite{Mutto2012LocallyCT} & -- & -- & -- & -- & 1.43 & 12.21 \\
        Dal Mutto et al. \cite{mutto2015probabilisticFusion} & -- & -- & -- & -- & 1.36 & 10.06 \\
        Ours & \textBF{0.26} & 2.14 & \textBF{0.67} & \textBF{4.10} & \textBF{0.45} & \textBF{1.52} \\
        \bottomrule
    \end{tabular}
    \vspace{-0.45cm}
\end{table}
\begin{table}[t]
	\centering
	\caption{\label{tab:plenoxels_vs_nerf}
        Plenoxels shows good novel view synthesis, but depth maps from Mip-NeRF are more accurate. Evaluated on the NeRF synthetic datasets~\cite{mildenhall2020nerf}.
    }	
    \begin{tabular}{l rr rrrr}
        \toprule
        \rule{0pt}{2.2ex} &  \multicolumn{2}{c}{Bad ratio (\%)} &  \multicolumn{4}{c}{Depth error}  \\
        & $>$0.2 & $>$0.05 & MAE Rel. & RMSE Rel.  & MAE & RMSE \\
        \midrule
        Plenoxels~\cite{yu2021plenoxels} & {11.84} & {55.84} & {0.032} & {0.139} & {0.120} & {0.275} \\
        Mip-NeRF~\cite{barron2021mipnerf} & {0.93} & {6.65} & {0.005} & {0.024} & {0.019} & {0.049} \\
        \bottomrule
    \end{tabular}
\end{table}

\mparagraph{Stereo+ToF Fusion Evaluation on other Datasets} 
We evaluate our fusion on SYNTH3 \cite{agresti2017fusion}, REAL3 \cite{agresti2019fusion_synthetic} and LTTM5 \cite{mutto2015probabilisticFusion}. 
Note that None of those datasets show the strong challenges encountered in the mobile environment, with higher power ToF modules and low distortion. In addition, their resolution is lower and raw ToF measurements are not provided, making the results not directly applicable to our phone.
However, they allow us to compare against numerous methods without reimplementation. 

SYNTH3 \cite{agresti2017fusion} dataset features 15 scenes rendered following \cite{Meister2013tofrender}. 
REAL3 \cite{agresti2019fusion_synthetic} features eight scenes captured with a ZED stereo camera and a Microsoft Kinect v2 ToF depth camera. Ground truth disparity is obtained with a line laser. 
LTTM5 \cite{mutto2015probabilisticFusion} consists of five scenes captured with two BASLER scA1000 RGB cameras and a MESA SR4000 ToF camera. Ground truth is acquired by spacetime stereo~\cite{zhang2003spacetime,Davis2005spacetime}. 
To accommodate for REAL3 and LTTM5's low RGB resolution, we linearly upsample the input stereo images two times in horizontal and vertical directions. 
Since ToF raw measurements are not available, we remove the confidence based on the difference between the estimated distance from the two frequencies. We also account for the intensity scale difference in the amplitude maps by setting $\sigma_A = 0.001$.
We present our results on these datasets in Table~\ref{tab:fusion_comparison} and on Figures \ref{fig:real3} and \ref{fig:lttm5}.

\mparagraph{Runtimes}
On our test system equipped with an NVIDIA RTX 3090, our online calibration takes 4.4 seconds and fusion takes 1.4 seconds.

\NEW{\mparagraph{Comparison against Plenoxels} Table~\ref{tab:plenoxels_vs_nerf} shows that Mip-NeRF~\cite{barron2021mipnerf} is better than Plenoxels~\cite{yu2021plenoxels} at estimating depth maps. We therefore use MipNeRF as a basis to generate training data.
}

\NEW{\mparagraph{Calibration Failure} Figure~\ref{fig:calibration_failure} shows an example of total calibration failure for Gao et al.~\cite{gao2017selfcalibratingtof}. Due to this, we use our calibration when comparing our fusion method against others in the main paper.
}

\bibliographystyle{splncs04}
\bibliography{bibliography}
